# Supplementary material for: Computing f-Divergences and Distances of High-Dimensional Probability Density Functions -- Low-Rank Tensor Approximations
Source: arXiv:2111.07164 source file (2022-09-07)
Supplement: Supplementary file 1 [file appendix.tex]

% !TEX root = ../19_low-rank_tensor_prob_den_char.tex
% !TEX encoding = UTF-8 Unicode

% RCSID:       $Id: appendix.tex,v 2.2 2022/05/18 23:48:22 hgm Exp $
% Authors:     Alexander Litvinenko, Youssef Marzouk, Hermann G. Matthies,
%              Marco Scavino, and Alessio Spantini
% Contact:     wire@tu-bs.de
% =================================

%% texfile{
%%  AUTHOR    = "$Author: hgm $",
%%  VERSION   = "$Revision: 2.2 $",
%%  DATE      = "$Date: 2022/05/18 23:48:22 $",
%%  FILENAME  = "$RCSfile: appendix.tex,v $"}

\appendix
\section{Appendix}
%\input{\thetext/TuckerFormat}
% !TEX root = ../19_low-rank_tensor_prob_den_char.tex
% !TEX encoding = UTF-8 Unicode

% RCSID:       $Id: notation_table.tex,v 2.1 2022/05/17 09:21:14 hgm Exp $
% Authors:     Alexander Litvinenko, Youssef Marzouk, Hermann G. Matthies,
%              Marco Scavino, and Alessio Spantini
% Contact:     wire@tu-bs.de
% =================================

%% texfile{
%%  AUTHOR    = "$Author: hgm $",
%%  VERSION   = "$Revision: 2.1 $",
%%  DATE      = "$Date: 2022/05/17 09:21:14 $",
%%  FILENAME  = "$RCSfile: notation_table.tex,v $"}

\begin{table}[h]
\caption{Notation}
\begin{tabular}{|c|l|}
\hline 
%\multicolumn{2}{|c|}{\textbf{General quantities}} \\ \hline
%${\Nset}$        &Natural numbers \\ \hline
%$(\Omega,\F{A},\D{P})$ & Probability space $\Omega$, $\sigma$-algebra $\F{A}$, and prob.\
% measure $\D{P}$ \\ \hline
$\vX$ & Random vector  $\vX=(\xi_1,...,\xi_d):\Omega\to\D{R}^d$ \\ \hline
$ \by$ & Parameter vector $ \by=(y_1,...,y_d)\in\D{R}^d$\\ \hline
\pdf & probability density function, denoted by $p_{\vX}(\by): \Rd\to\D{R}$ \\ \hline 
\pcf & probability characteristic function, denoted by $\vphi_{\vX}(\bt)$   \\ \hline 
$\bt$ & $\bt=(t_1,t_2,...,t_d) \in \D{R}^d$, the dual variable to $\by\in\Rd$ \\ \hline
\cdf & cumulative distribution function  \\ \hline RV & Random variable \\ \hline
KLD, $\widetilde{D}_{\text{KL}}$ & Kullback-Leibler divergence \\ \hline
$\EXP{\cdot}$ & expectation operator \\  \hline
$\bkt{\bt}{\by}$ & canonical Euclidean inner product on $\D{R}^d$,
   $\bkt{\bt}{\by}=\sum_{k=1}^d t_k y_k$ \\ \hline
%$\bx$ & vector $\bx=(x_1,...,x_d)$ \\ \hline
%$\bt$ & vector $\bt=(t_1,...,t_d)$ \\ \hline
$\tnb{P}$, $\tnb{Q}$ & tensors obtained after discretisation of two \pdfs \\ \hline 
% $\bar{\vX} = \EXP{\vX}\in\D{R}^d$ & mean value of random vector $\vX$  \\ \hline
% %$\tilde{\vX} = \vX - \bar{\vX}$ & mean zero part of random vector  $\vX$ \\ \hline
% $\F{B}$ & Borel $\sigma$-algebra of $\D{R}^d$ \\ \hline
% $\C{E}_{\by}\in\F{B}$ & semi-infinite interval in $\D{R}^d$, $\C{E}_{\by} = \bigtimes_{k=1}^d\;
%     ] \!-\!\infty, y_k ]$ \\ \hline
% $\mbf{1}_{\C{E}}(\by)$,  $\C{E}\in\F{B}$ & char./indicator function,  if $\by\in\C{E}$:
%   $\mbf{1}_{\C{E}}(\by) = 1$, else $\mbf{1}_{\C{E}}(\by) = 0$ \\ \hline
% $P_{\vX}(\C{E}) = \EXP{\mbf{1}_{\C{E}}(\vX)}$ & distribution (measure) of $\vX$
%      for $\C{E}\in\F{B}$, push forward $P_{\vX} = \vX_* \D{P}$ \\ \hline
% $F_{\vX}(\by) = P_{\vX}(\C{E}_{\by})$ & distribution fct.\ of $\vX$,
%      cumulative prob., $F_{\vX}(\by) = \D{P}(\vX \le \by)$ \\ \hline
% $p_{\vX}(\by)= \Di_{\by}F_{\vX}(\by)$ &  %($\Di_{\by}=\prod_{k=1}^d \dd_{y_k}$)
%   probability density fct.\ (\pdf) of $\vX$, and approximation $\tilde{p}_{\vX}(\by)$ \\ \hline
% $\vphi_{\vX}(\bt)=\EXP{\exp(\ii \ip{\bt}{\vX})}$   
%  & The characteristic fct.\ (\cdf)  of $\vX$, and approximation $\tilde{\vphi}_{\vX}(\bt)$\\ \hline
% $\chi_{\vX}(\bt)=\log(\vphi_{\vX}(\bt))$ & The 2nd characteristic or cumulant generating
%     fct.\ of $\vX$\\ \hline
% $\C{D}\subset\D{R}^d$ & Computational domain \\ \hline
% $I$, $I_N$ & Identity operator, identity matrix of size $N\times N$ \\ \hline
% %{KL}           & {Karhunen-Lo\`eve (Expansion)}\\ \hline
%(g)PCE            & (generalized) Polynomial Chaos Expansion \\ \hline
(i)(F)FT& (inverse) (Fast) Fourier transformation \\ \hline
$\iFd$, $\Fd$  & $d$-dimensional (inverse) Fourier transformation \\ \hline
%${\var}$           & Variance\\ \hline
%$H_{\alpha}$ & Multivariate Hermite polynomial with multi-index 
%  $\vek{\alpha}:=(\alpha_1,\ldots,\alpha_M)\in\D{N}_0^M$ & finite multi-index \\ \hline
%$h_{\alpha_m}(\theta_m)$ & univariate polynomial of variable $\theta_m$ \\ \hline
%$\alpha$, $\beta$, $\nu$ & multi-indices in gPCE\\ \hline
%$\J = \D{N}_0^{(\D{N})}$ & multi-index set \\ \hline
%$\vek{\alpha}$, $\vek{\beta}$, $\vek{\nu}\in\J$ & multi-indices 
%   $\vek{\beta}:=(\beta_1,\ldots,\beta_{M},...)$\\ \hline
%$\J_{M,p}\subset\D{N}_0^M\subset\J$ & $M$ components, max.\ polynomial order $p$\\ \hline
%$L$ & Number of the KLE terms after truncation \\ \hline
%$M$ & Stochastic dimension \\ \hline
%$d$ & dimension of $\vX$ \\ \hline
% $\param$ & high-dimensional parameter \\ \hline
%$p$ & polynomial order or vector of them, $\vek{p}=(p_1,\ldots,p_M)$ \\ \hline 
%\multicolumn{2}{|c|}{\textbf{Multidimensional and/or tensor product quantities}} \\ \hline
%{TT}           & Tensor train data format \\ \hline
$\otimes$  & Tensor (Kronecker) product \\ \hline
QoI & Quantity of Interest \\ \hline
%$\times$  & Cartesian product \\ \hline
%$u(\theta_1,\ldots,\theta_M)$ & $M$-variate function \\ \hline
%$ \bTheta_{\vek{\gamma}}= \bigtimes_{\ell=1}^M \theta_{\gamma_{\ell}}$ & $M$-dimensional grid 
% $\vek{\gamma}=(\gamma_1,...,\gamma_M),\,\, \theta_{\gamma_{\ell}}=(1,...,n_{\gamma_{\ell}})$ 
% \\ \hline
%$\mT$ & $d$-dim. grid, $=\bigotimes_{\ell=1}^d \tau_{\ell}\in \mathbb{R}^{n_1\times n_2 ... 
%  \times n_d},\,\quad \tau_{\ell}\in \mathbb{R}^{n_{\ell}}$ 
%\\ \hline
\end{tabular}
\label{tab:notations}
\end{table}%
%

%  $Log: notation_table.tex,v $
%  Revision 2.1  2022/05/17 09:21:14  hgm
%  in rev 2
%
%  Revision 1.2  2021/11/07 22:34:04  hgm
%  added header and footer
%
%  Revision 1.12  2021/11/07 22:19:10  hgm
%  added header and footer
%
%
%
%
%
%

%%% Local Variables: 
%%% mode: latex
%%% TeX-master: "../19_low-rank_tensor_prob_den_char"
%%% End: 

%\subsection{Matlab code for TT approximation of $d$-variate \pcf}
%\label{sec:matlabcode}

%

%  $Log: appendix.tex,v $
%  Revision 2.2  2022/05/18 23:48:22  hgm
%  still shortening
%
%  Revision 2.1  2022/05/17 15:17:52  hgm
%  for V2
%
%  Revision 1.12  2021/11/07 22:23:31  hgm
%  added header and footer
%
%  Revision 1.12  2021/11/07 22:19:10  hgm
%  added header and footer
%
%
%
%
%
%

%%% Local Variables: 
%%% mode: latex
%%% TeX-master: "../19_low-rank_tensor_prob_den_char"
%%% End: 
