# Supplementary material for: Computing f-Divergences and Distances of High-Dimensional Probability Density Functions -- Low-Rank Tensor Approximations
Source: arXiv:2111.07164 source file (2022-09-07)
Supplement: Supplementary file 2 [file appendix_old.tex]

% !TEX root = ../19_low-rank_tensor_prob_den_char.tex
% !TEX encoding = UTF-8 Unicode

% RCSID:       $Id: appendix.tex,v 1.12 2021/11/07 22:23:31 hgm Exp $
% Authors:     Alexander Litvinenko, Youssef Marzouk, Hermann G. Matthies,
%              Marco Scavino, and Alessio Spantini
% Contact:     wire@tu-bs.de
% =================================

%% texfile{
%%  AUTHOR    = "$Author: hgm $",
%%  VERSION   = "$Revision: 1.12 $",
%%  DATE      = "$Date: 2021/11/07 22:23:31 $",
%%  FILENAME  = "$RCSfile: appendix.tex,v $"}


\appendix
\section{Appendix}
%\input{\thetext/TuckerFormat}

\subsection{Matlab code for TT approximation of $d$-variate \pcf}
\label{sec:matlabcode}
In this example a given $d$-dimensional multivariate functions 
(e.g., a $d$-dimensional elliptically contoured stable 
distribution as in Example~\ref{ex:biVarEllip}) for general $d$ is approximated in the TT data format. To be able to run the code below the 
TT-toolbox\footnote{https://github.com/oseledets/TT-Toolbox.git} should be installed. 
%
\begin{lstlisting}
d = 8;
n = 512;
a = 128;
x = (-a+2*a/n:2*a/n:a)';
freq = (-pi/(x(2)-x(1))+2*pi/(2*a):2*pi/(2*a):pi/(x(2)-x(1)))';
fft_magn = n*sqrt(2*pi)/(2*a);
P = sparse(n,n);
P(1:n/2, n/2:-1:1) = speye(n/2);
P(n/2+1:n, n:-1:n/2+1) = speye(n/2);
tol = 1e-6;
alpha=1.0; % working for alpha={0.7, 1.0, 1.5, 2.0}
mu = 1.1.*(1:d)'
gfun = @(x)exp(1i*x*mu -sqrt(sum(x.^2,2)/2).^alpha) / (2*pi)^(d/2);
g0 = tt_unit(n,1,n/2);
g0 = mtkron(repmat({g0}, 1, d));
g = amen_cross_s(n*ones(d,1), @(ind)gfun(reshape(x(ind), [], d)), tol, 
'vec',true, 'y0', g0);
f = g;
for i=1:d
        fi = f{i}; % dimensions r1 x n x r2
        [r1,~,r2] = size(fi);
        fi = permute(fi, [2,1,3]);
        fi = reshape(fi, n, r1*r2);
        fi = P*fi;
        fi = ifft(fi);
        fi = fi/(fft_magn/n);
        fi = P*fi;
        fi = reshape(fi, n, r1, r2);
        fi = permute(fi, [2,1,3]);
        f{i} = fi;
end
error = dot(tt_ones(n,d)/n^d, f)*(2*pi/(x(2)-x(1)))^d - 1
\end{lstlisting}
%
% Assume that $\vphi_{\vX}(\bt)$ can be approximated by means of low-rank tensor techniques as follows:
% \begin{equation}
% \vphi_{\vX}(\bt)\approx \tilde{\vphi}_{\vX}(\bt)=
%   \sum_{\ell=1}^R\Ten_{\mu=1}^d \vphi_{\ell,\mu}(t_\mu).
% \end{equation}
%
%Factors $\varphi_{\ell,\nu}(t_\mu)$ may not have properties of the 
%characteristic function. But this is not an issue here, since these factors are only auxiliary functions.  The most important is 
%$\tilde{\vphi}_{\vX}(\bt)$, which can be computed with any accuracy $\vepsilon$: 
%$\Vert {\vphi}_{\vX}(\bt) - \tilde{\vphi}_{\vX}(\bt) \Vert \leq \vepsilon$.

%Examples could be the $d$-dimensional Cauchy distribution, and 
%the $d$-dimensional elliptically contoured stable distribution.



% \subsection{Connection of PCE, \pdf and \pcf}
% \textcolor{red}{HM: Here we explain how to get from RV $\xi$ in a low-rank format to \pcf or moment generating function, all in low-rank.}

% %
% \begin{align}  \label{eq:motiv_inv3}
% p_{\vX}(\by)&= \frac{1}{(2\uppi)^d} \int_{\D{R}^d}\exp(-\ii\ip{\by}{\bt})
%   \vphi_{\vX}(\bt) \di \bt \\  \nonumber
% &\approx  \int_{\D{R}^d}\exp(-\ii \sum_{j=1}^d y_{j}t_{j})
% \sum_{\ell=1}^R \Ten_{\mu=1}^d \vphi_{\ell,\mu}(t_\mu)
% dt_1...dt_d \\ \nonumber
% &\approx \sum_{\ell=1}^R  \Ten_{\mu=1}^d \int_{\D{R}}\exp(-\ii\, y_{\mu} t_{\mu})
%   \vphi_{\ell,\mu}(t_{\mu}) \di t_{\mu} 
% \approx \sum_{\ell=1}^R \Ten_{\mu=1}^d p_{\ell, \mu}(y_{\mu}).
% \end{align}
% Further we computed numerically a low-rank approximation of the 
% $d$-variate elliptically contoured $\alpha$-stable distribution. \AL{Further we fix $\alpha=0.5$ and compute divergences from Table~\ref{table:divergences-discr}.}
%\mbox{http://www.mathematik.uni-ulm.de/stochastik/lehre/ws02_03/statistik_2/skript/node25.html}
%\end{example}

% \textbf{Bivariate Cauchy distribution}. If we set $d=2$ and $\alpha=1/2$ in \eqref{eq:motiv_ch2}, then we obtain the well-known bi-variate 
% Cauchy distribution.
% It is not analytically separable, but it is possible to find a numerical rank-$k$ approximation. One can use the SVD algorithm or some heuristics.


%
% \AL{Further we compute distances $D_{KL}$ and $D_{H^2}$ between two $d$-variate elliptically contoured $\alpha$-stable distributions with $\alpha=1$ and $\alpha=2$. The mean values and matrices $\Sigma$ are assumed to be equal. All Table as in previous example. TODO}

% \begin{table}[htbp!]
%  \centering
%  \begin{tabular}{|l|l|l|l|l|l|}
%  \hline
% %$D_{\text{KL}}(\mathcal{N}_1\vert \mathcal{N}_2)$ &  & \\ \hline \hline
% $(\alpha_1, \alpha_2)$ & $(2.0,0.5)$ &$(2.0,1.0)$ &$(2.0,1.5)$ & $(1.0,0.9)$& $(1.5,1.4)$\\ \hline
% $D_{\text{KL}}(\alpha_1,\alpha_2)$ & negative & \textcolor{red}{negative -0.38} & -0.3 & -0.025 & -0.03 \\ \hline
% comp. time, sec. &  &  && & \\ \hline
% max. TT rank &  & && & \\ \hline
% memory. req. in MB  &  &  && & \\ \hline

% %Bregman divergence  --- $D_{\phi}$:	&&&\\ \hline
% %Bhattacharyya distance --- $D_{\text{Bh}}$: &&& \\ \hline
% \end{tabular}
%  \caption{Computation of $D_{\text{KL}}(\alpha_1,\alpha_2)$ between two $\alpha$ -stable distributions for fixed $d=16$ and $n=64$. TT cross algorithm with tolerance $10^{-12}$ is used.}
%  \label{table:divergences-comput_alpha_KLD_d8}  
% \end{table}%


%  $Log: appendix.tex,v $
%  Revision 1.12  2021/11/07 22:23:31  hgm
%  added header and footer
%
%  Revision 1.12  2021/11/07 22:19:10  hgm
%  added header and footer
%
%
%
%
%
%



%%% Local Variables: 
%%% mode: latex
%%% TeX-master: "../19_low-rank_tensor_prob_den_char"
%%% End: 
