# Supplementary material for: Computing f-Divergences and Distances of High-Dimensional Probability Density Functions -- Low-Rank Tensor Approximations
Source: arXiv:2111.07164 source file (2022-09-07)
Supplement: Supplementary file 3 [file appendix_old_full.tex]

% !TEX root = ../19_low-rank_tensor_prob_den_char.tex
% !TEX encoding = UTF-8 Unicode

% RCSID:       $Id: appendix.tex,v 1.10 2021/08/03 08:24:00 hgm Exp $
% Authors:     Alexander Litvinenko, Youssef Marzouk, Hermann G. Matthies,
%              Marco Scavino, and Alessio Spantini
% Contact:     wire@tu-bs.de
% =================================

%% texfile{
%%  AUTHOR    = "$Author: hgm $",
%%  VERSION   = "$Revision: 1.10 $",
%%  DATE      = "$Date: 2021/08/03 08:24:00 $",
%%  FILENAME  = "$RCSfile: appendix.tex,v $"}

\appendix

\section{Appendix}
%\input{\thetext/TuckerFormat}

%\input{\thetext/common_notation}
%\input{\thetext/notation_table}
%\input{\thetext/distances}

% \subsection{TO DELETE: Computing \pcf from RV $\vX(\thetab)$}
% We start with RV $\vX(\thetab)$ given as in \eqref{eq:KLE-PCE-d} and compute \pcf $\vphi_{\vX}(\bt)$ by formula in \eqref{eq:pcf1}.
% We take the dual grid for parameter $t$, defined in Section \ref{SSS:discr-low-rank-dens-char-DFT}, compute scalar product between two tensors as in \eqref{eq:CP_scalarProd}, and
% as a results, obtain a \pcf tensor $\tnb{\Phi}:= (\tns{\Phi}_{i_1,\dots,i_d}) = \vphi_{\vX}(\That{T})$ as in \eqref{eq:grid-char}-\eqref{eq:FT-char-cont-LR}.


%\newpage
\subsection{Matlab code for TT approximation of $d$-variate \pcf}
\label{sec:matlabcode}
In this example a given $d$-dimensional multivariate functions 
(e.g., a $d$-dimensional elliptically contoured stable 
distribution as in Example~\ref{ex:biVarEllip}) for general $d$ is approximated in the TT data format. To be able to run the code below the 
TT-toolbox\footnote{https://github.com/oseledets/TT-Toolbox.git} should be installed. 
%
\begin{lstlisting}
d = 8;
n = 512;
a = 128;
x = (-a+2*a/n:2*a/n:a)';
freq = (-pi/(x(2)-x(1))+2*pi/(2*a):2*pi/(2*a):pi/(x(2)-x(1)))';
fft_magn = n*sqrt(2*pi)/(2*a);
P = sparse(n,n);
P(1:n/2, n/2:-1:1) = speye(n/2);
P(n/2+1:n, n:-1:n/2+1) = speye(n/2);
tol = 1e-6;
alpha=1.0; % working for alpha={0.7, 1.0, 1.5, 2.0}
mu = 1.1.*(1:d)'
gfun = @(x)exp(1i*x*mu -sqrt(sum(x.^2,2)/2).^alpha) / (2*pi)^(d/2);
g0 = tt_unit(n,1,n/2);
g0 = mtkron(repmat({g0}, 1, d));
g = amen_cross_s(n*ones(d,1), @(ind)gfun(reshape(x(ind), [], d)), tol, 
'vec',true, 'y0', g0);
f = g;
for i=1:d
        fi = f{i}; % dimensions r1 x n x r2
        [r1,~,r2] = size(fi);
        fi = permute(fi, [2,1,3]);
        fi = reshape(fi, n, r1*r2);
        fi = P*fi;
        fi = ifft(fi);
        fi = fi/(fft_magn/n);
        fi = P*fi;
        fi = reshape(fi, n, r1, r2);
        fi = permute(fi, [2,1,3]);
        f{i} = fi;
end
error = dot(tt_ones(n,d)/n^d, f)*(2*pi/(x(2)-x(1)))^d - 1
\end{lstlisting}
%
% \subsection{Connection of PCE, \pdf and \pcf}
% \textcolor{red}{HM: Here we explain how to get from RV $\xi$ in a low-rank format to \pcf or moment generating function, all in low-rank.}



%Among other things, we try to answer on the following questions. 1) 
\textcolor{red}{Assuming PCE of a given RV is expressed in a low-rank tensor format, what can we say about low-rank approximability of its \pdf? 2) its \pcf?}
\textcolor{red}{NEW. In \cite{Waehnert14} tensor ranks of RVs and random fields (RFs), representing random coefficients and operators of a stochastic elliptic PDE,  were investigated. In \cite{ESHALIMA11_1}
it was shown how to compute level sets and then the histograms if the PCE of the RV is given in a low-rank tensor format. Thus, these two works may help to give a positive answer on the first question, i.e., if PCE of the RV is approximated by a tensor of a low rank, then there are numerical methods, which under certain assumptions, can compute its \pdf also in a low-rank tensor format. Additionally, \pcf and \pdf are connected via (inverse) Fourier Transform, which has the tensor rank 1, meaning, that the answer on the second question could be positive too.}

Below we provide low-rank tensor approximations of various
\pcfs and \pdfs.
%and demonstrate how to compute mixed higher order moments. 
% We remind that if a random variable has symmetric zero-mean distribution, 
% then the corresponding characteristic function is a real function, with 
% zero complex component.

\paragraph{Discretisation.}
Let us discretise the physical space (in 1D) and the frequency space. Setting $\vX=\xi$, $\by=y$, and $\bt=t$, we obtain
\begin{equation}  \label{eq:p_ten3}
p_{\xi}(y)=:p(y)=\frac{1}{\uppi}\int_{0}^{\infty}\exp(-\ii yt)
  \varphi(t)\di t.
\end{equation}
Let us introduce a mesh for $\bt$ and approximate this integral above via a finite sum. We define $t=\eta\cdot (j-1)$, $j=1..n$, then
\begin{equation}  \label{eq:p_ten_desc}
p(y)\approx \frac{1}{\uppi}
\sum_{j=1}^n 
\exp(-\ii y \eta\cdot (j-1))
  \varphi(t_j)\eta.
\end{equation}
Then
$y_k=-\frac{1}{2}N\lambda (k-1)=-b+\lambda(k-1)$, and
\begin{equation}  \label{eq:p_ten_desc2}
p(y_k)\approx \frac{1}{\uppi}
\sum_{j=1}^n 
\exp(-\ii \lambda\eta(k-1)(j-1))\cdot \exp(ibs_j)
  \varphi(t_j)\eta.
\end{equation}
Here we chose parameters $\lambda$ and $\eta$ so that: $\lambda\eta=\frac{2\pi}{n}$:
\begin{equation}  \label{eq:p_ten_desc3}
p(y_k)\approx 
\sum_{j=1}^n 
\exp(-\ii \frac{2\uppi}{n}(k-1)(j-1))\cdot \exp(ibs_j)
  \varphi(t_j)\eta,
\end{equation}
where $b=\frac{N\lambda}{2}$ and $s=\eta(j-1)$.
Later, to compute \pdf,  we will apply the FFT procedure to the argument $\exp(ibs_j)\varphi(t_j)\eta$.
%
\subsection{Candidate to be deleted: Error analysis}

%
%Let $\Fd$ be the $d$-dimensional Fourier transform and %$\iFd$ the $d$-dimensional 
%inverse Fourier transform. 
% \ALs{\begin{proposition}
% Let $\vX$ be a $d$-dimensional random variable, whose density $ p_{\vX}(\by)$ exists. 
% Let $\varphi_{\vX}(\bt)$ be its corresponding $d$-dimensional characteristic function, 
% and assume that there is a low-rank tensor approximation of $\vphi_{\vX}(\bt)$, such 
% that  
% \begin{equation}  \label{eq:err_phi}
% \Vert \vphi_{\vX}(\bt) - \sum_{\ell=1}^R\Ten_{\mu=1}^d \vphi_{\ell,\mu}(t_\mu)\Vert_2 
%   \leq \vepsilon.
% \end{equation}
% %
% Then
% \begin{equation}  \label{eq:err_f}
% \Vert p_{\vX}(\by)-\sum_{\ell=1}^R \Ten_{\mu=1}^d p_{\ell, \mu}(y_{\mu})\Vert_2 \leq \vepsilon.
% \end{equation}
% \end{proposition}
% \begin{proof}
% \begin{align*}  \label{eq:err_proof}
% \Vert p_{\vX}(\by)-\sum_{\ell=1}^R \Ten_{\mu=1}^d p_{\ell, \mu}(y_{\mu})\Vert_2 =
% \Vert \iFd (\vphi_{\vX}(\bt)) - \iFd \left (\sum_{\ell=1}^R
% \Ten_{\mu=1}^d \vphi_{\ell,\mu}(t_\mu)\right)\Vert_2 &\leq \\ \nonumber
% \leq \Vert \iFd \Vert \cdot \Vert \vphi_{\vX}(\bt) - \sum_{\ell=1}^R\Ten_{\mu=1}^d 
% \vphi_{\ell,\mu}(t_\mu)\Vert_2 \leq 1\cdot \vepsilon.
% \end{align*}  
% \end{proof}}

%
\begin{remark}
Generally speaking, a low-rank approximation of the probability density function is 
not a probability density function, but we can achieve any prescribed 
approximation accuracy.  In the worst case we must take the full rank.
\end{remark}
\ALc{THIS TEXT BELOW repeats what we have already written earlier. HM wanted to combine it with Introduction.} However, after appropriate scaling, numerical low-rank approximations of characteristic and density 
functions can still serve as characteristic and density functions.
For the \pdf,  we should fulfil two conditions: it
should be non-negative (for each value) and the integral should be equal one. 
The second requirement can be achieved by normalisation. 
The mentioned above restrictions are very general in the low-rank theory.
For example, permeability, conductivity, porosity coefficients in PDEs are physical 
values and can not be negative, but during low-rank approximation they may become 
negative.  To avoid it, a constrained optimisation problem is solved. 
The ``constrained'' means that the solution lives on some manifold and 
should stay on this manifold during the whole computing process. 
One of the possible remedies is introduction of  a new projection operator, 
which returns the solution back to the manifold, once it leaves this manifold.
%\textcolor{red}{TO ADD MORE DETAILS ABOUT TRUNCATION. Non-Closed set, Newton method, etc }.

\subsubsection{Computing cost and storage}
In many chemical applications one has $n=100$, and $d$ is few hundreds or even 
thousands \citep{MikeRaoKhor}.
Some other high-dimensional problems from chemistry and physics like 
Hartree-Fock$-,$ Schr\"odinger$-,$ or Master$-$equations, and low-rank tensor methods 
of their solution are for example considered in 
\citep{KhorSurvey, khoromskaia2018tensor, khorBook18, Dolgov_Master},
see also the references therein.
Another example of large volumes of high-dimensional data are  
satellite data.  Satellites collect data over a very large areas (e.g.\ the data collected 
by the National Center for Atmospheric Research (USA) \citep{GrossmanMazzucco2002}.
%\footnote{\url{https://www.earthsystemgrid.org/}}). 
Big data can also come from a computer simulator codes such as a solution of a
multi-parametric equation, e.g.\ weather research and forecasting, and
climate models \citep{Eyring2019}.  Also
%model\footnote{\url{https://www.mmm.ucar.edu/weather-research-and-forecasting-model}}). 
Oil$\&$Gas companies daily collect sensor
data from multiple sources.  
Another source for huge volumes of data are high-energy
particle accelerators like CERN \citep{Brumfiel2011}.


\subsubsection{DECIDED TO DELETE, WE HAVE IT ALREADY. Reshaping of the vector}
A tensor is a multi-index 
array, where multi-indices are used instead of indices.  As an
example, consider a vector
$\vek{w}\in\D{R}^N$, $N=10^{12}$ data points.  We can \emph{reshape}
it into a matrix $\vek{W}\in\D{R}^{10^6 \times 10^6}\cong \D{R}^{10^6}\otimes\D{R}^{10^6}$, which is 
a tensor of 2nd order. To get a tensor of 3rd order, we reshape it in the following way
$\D{R}^{10^4 \times 10^4 \times 10^4}\cong \bigotimes_{k=1}^3 \D{R}^{10^4}$ and so on (see Section 1 in \cite{Matthies2020}).
%One way to obtain a tensor
%from a vector or matrix is to reshape it.  For example, 
%assume $\vek{v} \in \D{R}^{10^6}$ is a vector. After reshaping it
%we can obtain a matrix --- a tensor of 2nd order --- of size $10^3 \times 10^3$, 
%or a tensor of 3rd order of size $10^2\times 10^2\times 10^2$,
% or a tensor of 6th order of size $10\times ... \times 10$ (6 times). 
%Each element of such a six-dimensional hypercube is described by a multi-index 
%$\vek{m}=(m_1,\dots,m_6)$. 
The higher the order of the tensor, the more possibilities there are to find
a low-rank approximation \citep{HA12}.
The tensors  obtained in this way contain not only rows and columns, but also
\emph{slices} and \emph{fibres} \citep{Kolda:01, Kolda:07, DMV-SIAM2:00, HA12}. 
These slices and fibres can be analysed for linear dependencies, super symmetry,
or sparsity,  and may result in a strong data compression \cite{WhyLowRank19}.  
%!!!

\subsubsection{(Decided to delete it. Check!) Algebra}
\ALc{ THIS TEXT BELOW IS COPIED} 
The set of possible objects we want to work with will be denoted by $\C{T}$.
We assume that this set is equipped with the operations of an associative and
commutative real algebra, and carries an inner product.  It is a well known result
\citep{Segal1978} that such algebras --- modulo some technical details --- are
isomorphic via the Gel'fand representation to a function algebra --- 
to be more precise continuous real valued functions on a compact set.  
Under point-wise addition and multiplication by scalars, such functions
clearly form a vector space, and if one includes point-wise multiplication of functions,
they form an associative and commutative real algebra.  In our case this is simply
the function algebra $(\C{M}=\bigtimes_{\ell=1}^d \{1,\dots,M_\ell \} \to \D{R})$, 
which is obviously the same as $\bigotimes_{\ell=1}^d \D{R}^{M_\ell}$.
The advantage of this abstract algebraic formulation is not only that it
applies to any kind of data representation on which one may define these algebraic
operations, but that one may use algorithms \citep{NHigham} which have been developed
for the algebra of real $N\times N$ matrices $\F{gl}(\D{R},N)
= \D{R}^{N \times N} \cong \D{R}^N\otimes\D{R}^N$.\\
In our concrete examples we work directly with the data represented as tensors
$\C{T}:= \bigotimes_{\ell=1}^d \D{R}^{M_\ell}$.  Even without the identification
with $(\C{M} \to \D{R})$, it is obvious that this is naturally a vector space.  
As also $\C{T}\cong \D{R}^N$, it is clear that $\C{T}$ can be equipped with 
the canonical Euclidean inner product from $\D{R}^N$.  The associative and 
commutative algebra product comes from the identification with the function 
algebra $(\C{M} \to \D{R})$, i.e.\ the point-wise product, which is also known
as the \emph{Hadamard} product \citep{HA12}.  Hence it is clear that for 
data $\vek{w}\in\D{R}^N$ it is not difficult at all to define the algebraic 
operations, but rather how to perform them when the data is in a compressed format.\\
To simplify later notation on the number of operations and amount of storage
needed, we will often make the assumption that $M_1 = \dots = M_d = n$, so that the
tensor in \refeq{eq:CPI} represents $N=n^d$ values.
As already mentioned, our example of data compression is based on
low-rank approximations to elements in $\C{T}$.
Although low-rank tensor data formats and techniques are almost
unavoidable if working with large high-dimensional data sets,
we would like to stress that the algorithms presented here are
formulated purely in terms of the abstract algebraic structure,
and are thus independent of the particular representation.\\
Whereas a general element $\tnb{w}\in\C{T}$ hence has $N=n^d$ terms,
a compressed representation --- some low-rank versions of which
will be discussed in more detail in \refS{tensor-rep} --- will have
significantly fewer terms.  For example, the \emph{CP}-decomposition
(\emph{canonical polyadic}) representation, truncated to $r$ terms,
\begin{equation}  \label{eq:CPI}
   \tnb{w} \approx \tnb{w}_r = \sum_{i=1}^r   \bigotimes_{k=1}^d 
     \vek{w}_{i,k}; \;  \vek{w}_{i,k} \in \D{R}^{n},\; \text{has }\,
    r\times n \times d \; \text{terms in}\; \tnb{w}_r.
\end{equation}
The reduced SVD is a special case of \refeq{eq:CPI}, where the
required storage is reduced from $N=M^2$ to $2\times r\times M$ units.
If the \emph{rank} $r$ is reasonably small compared to $N=n^d$ independent of $n$ and $d$,
then we have an approximation $\tnb{w}_r\in\C{T}$ with much less storage, which also
only depends on the \emph{product} of $n$ and $d$ and is not exponential in the
dimension $d$.  But now the maximum can not
be easily looked up; to get a particular element, the expression \refeq{eq:CPI}
has to be evaluated for that index combination.  In the following
we shall assume that we work with approximations such as in \refeq{eq:CPI}
which need much less storage.  One has to make sure then that the \emph{algebraic}
operations of the Hadamard algebra structure on $\C{T}$ can be performed efficiently
in an approximative manner, so that they
have much lower complexity than the obvious $\C{O}(n^d)$, although
the single elements of $\tnb{w}$ which are usually needed for point-wise operations
--- and post-processing, see \ref{S:statistics} --- are not directly available.


\begin{example}[Approximation of $d$-variate Gaussian distribution]
\textcolor{red}{REPEATED. To delete !}
Let $\vphi_{\vX}(\bt)$ be a $d$-dimensional Gaussian random vector 
$\vX=(\xi_1,\xi_2,...,\xi_d)$ with the mean $\mu=(\mu_1,\mu_2,...,\mu_d)^\trpos$ 
and the diagonal covariance matrix  $\bC=\diag(\sigma_1^2,\ldots,\sigma_d^2)$.
The corresponding characteristic function is
\begin{equation}
\vphi_{\vX}(\bt)=\exp \left( \ii(t_1,\ldots,t_d)\cdot (\mu_1,\ldots,\mu_d)^\trpos -
  \frac{1}{2}(t_1,\ldots,t_d)
\Sigma
(t_1,\ldots,t_d)^\trpos
\right).
\end{equation}
One can see that $\vphi_{\vX}(\bt)$ is separable and has the tensor rank 1, i.e.\
\begin{equation}
\vphi_{\vX}(\bt)=\exp \left( \ii t_1 \mu_1-\frac{1}{2}\sigma^2_1 t_1^2 \right)
  \cdot ... \cdot
\exp \left( \ii t_d \mu_d-\frac{1}{2}\sigma^2_d t_d^2 \right)=
\prod_{\nu=1}^d \vphi_{\xi_{\nu}}(t_{\nu}).
\end{equation}
%
Further, from the inversion theorem \cite{Lukacs70b}, the \pdf of 
$\vX$ on $\D{R}^d$ can be computed from $\vphi_{\vX}(\bt)$ as follows 
% \begin{equation}  \label{eq:motiv_inv}
% p_{\vX}(\by)=\frac{1}{(2\uppi)^d} \int_{\D{R}^d}
%   \exp(-\ii\ip{\by}{\bt})\vphi_{\vX}(\bt)\di\bt, \quad \by \in \D{R}^d
% \end{equation}
% or
\begin{align*}  \label{eq:motiv_inv2}
p_{\vX}(\by)&=\frac{1}{(2\uppi)^d}\int_{\D{R}^d}\exp(-\ii \ip{\by}{\bt})
  \vphi_{\vX}(\bt) \di\bt \\
%&=\frac{1}{(2\uppi)^d}\int_{\D{R}^d}\exp(-\ii (y_1 t_1 +...+y_d t_d))
%  \vphi_{\xi_1}(t_1)...\vphi_{\xi_d}(t_d)\di t_1...\di t_d\\
&=\frac{1}{2\uppi}\int_{\D{R}}\exp(-\ii y_1 t_1)\vphi_{\xi_1}(t_1)\di t_1 \cdot ...\cdot
\frac{1}{2\uppi}\int_{\D{R}}\exp(-\ii y_d t_d)\vphi_{\xi_d}(t_d)\di t_d \\
&=:p_{\xi_1}(y_1) \cdot ... \cdot p_{\xi_d}(y_d),\quad \by:=(y_1,\ldots,y_d) \in \D{R}^d.
\end{align*}
\end{example}
Observe that the probability density $p_{\vX}(\by)$ is analytically separable and is expressed as a product of $d$ uni-dimensional densities.

The \emph{differential entropy} (see \refeq{eq:discr-diff-entrop}), requiring the 
point-wise logarithm of $p$, will be:
\begin{align*} 
   h(p) &:= \EXP{-\ln(p_{\vX}(\by))} = \EXP{-\ln(p_{\xi_1}(y_1) \cdot ... \cdot p_{\xi_d}(y_d))}=-\sum_{\nu=1}^d \EXP{\ln(p_{\xi_{\nu}}(y_{\nu}))}.
%   &=-\EXP{\log(p_{\xi_1}(y_1)) }- \ldots - \EXP{\log(p_{\xi_d}(y_d))}.
\end{align*}
i.e. for the $d$-dimensional Gaussian case, the differential entropy is a sum of one-dimensional entropies. Here we must receive the well known formula for computing differential entropy of $d$-dimensional Gaussian random vector:
\begin{equation*}
    \hat{h}(p)=\frac{n}{2}+\frac{n}{2}\ln(2\pi)+\frac{n}{2}\ln(|\bC|).
\end{equation*}
This example with analytically known entropy is useful to demonstrate the whole approach. After estimating \pdfs from \pcfs, computing pointwise logarithms, we should obtain $h(p)\approx \hat{h}(p)$.


\begin{example}
The KL divergence for two \AL{ADD DEFINITION spherically contoured $\gamma$-order normally distributed RVs} with the same mean and shape parameter $\gamma$ is given by
\begin{equation}
\label{eq:gammaKLD}
    D_{KL}(X\Vert Y)=d\log \frac{\sigma_2}{\sigma_1} - d\left (\frac{\gamma-1}{\gamma} \right)
    \left[ 
    1-\left(\frac{\sigma_1}{\sigma_2} \right)^{\frac{\gamma}{\gamma-1}}
    \right ].
\end{equation}
Here $X:=(X_1,\ldots,X_d)\sim  \mathcal{N}_{\gamma}(\mu_1,\sigma_1^2I_d)$ and 
$Y:=(Y_1,\ldots,Y_d)\sim  \mathcal{N}_{\gamma}(\mu_2,\sigma_2^2I_d)$, $\mu=\mu_1=\mu_2 \in \mathbb{R}^d$ \cite{Kitsos_2010,Toulias2020}. If $\gamma=2$ and $\mu_1\neq\mu_2$, then we receive the usual KL divergence from one normally distributed RV to another
\begin{equation}
\label{eq:dKLD}
       D_{KL}(X\Vert Y)=\frac{d}{2}\left[ 2\log \frac{\sigma_2}{\sigma_1} - 1+ \left (\frac{\sigma_1}{\sigma_2} \right)^2+\frac{\Vert \mu_2-\mu_1\Vert^2}{d\sigma_2^2}
    \right].
\end{equation}
Now we will use both formulas \refeq{eq:dKLD} and \refeq{eq:gammaKLD} as the reference solution. First, we will use iterative algorithms (and the low-rank tensor format technique) to compute KLD from \refeq{eq:dKLD} for $d=2$, and then KLD from \refeq{eq:gammaKLD}.
\end{example}
We fixed parameters $\gamma=2$, $\mu_1=\mu_2=5$, $\sigma_1=1$, $\sigma_2=2$ and computed the KLD by the classical MC and by Eq.~\ref{eq:KLDgamma}. The first value is $63.6783$ and the second $63.6294$.

%
%
%
\subsection{Numerical computation of $f$-divergences}
\ALc{THIS WILL BE A  NEW SECTION. TO BE DONE.}\\
In this section we compute numerically 
the divergences listed in Table~\ref{table:divergences-discr}.
We use low-rank tensor formulas from  Sections~\ref{S:theory} and \ref{SSS:iter-fcts},  classical Monte Carlo and analytical formulas if available. The last two approaches are used for validation purposes. The results are summarized in Table~\ref{table:divergences-comput}:

\begin{table}[h]
 \centering
 \begin{tabular}{|l|l|l|l|}
 \hline
Name of the divergence & Tensors & MC & Analytical \\ \hline \hline
Kullback–Leibler-(KL) --- $D_{\text{KL}}$: &&&\\ \hline
squared Hellinger distance --- $D_{H^2}$: &&& \\ \hline
%Bregman divergence  --- $D_{\phi}$:	&&&\\ \hline
%Bhattacharyya distance --- $D_{\text{Bh}}$: &&& \\ \hline
\end{tabular}
 \caption{Numerical computations of $f$-divergences, computed by low-rank tensors methods, MC method, and by analytical formulas respectively. \ALc{TO BE DONE. COMPUTE TIME}}
 \label{table:divergences-comput}  
\end{table}
%
\ALc{We see the following advantages by applying low-rank tensor techniques and not classical sampling methods like Monte Carlo: 1) by low-rank tensors the computational complexity is $\mathcal{O}(dr\log N)$, $d,r$ small integers, whereas by MC $\mathcal{O(N)}$; 2) we obtain a low-rank tensor representation naturally after applying, e.g., the stochastic Galerkin method \citep{Zander10, matthiesKeese05cmame, SchwabKLE, ullmann-diss, dolgov2015polynomial, dolgov2014computation}; 3) it is time-consuming or even impossible to compute divergences in high-dimensions via MC; 4) we replace random sampling error (in MC) by deterministic truncation error, which can be better controlled; 5) we improve the convergence rate, which is $\mathcal{O}({{N}^{-1/2}})$ by MC.}




\begin{example}[family of the elliptically contoured $\gamma$-order generalized normal distributions]
The $d$-variate random variable $\vX$ follows the $\gamma$-order generalized normal distribution ($\gamma$-GND) \cite{Toulias2020}, i.e., $\vX \sim \mathcal{N}^d_{\gamma}(\mu,\Sigma)$ 
with the mean vector (also known as the location parameter vector) $\mu \in \mathbb{R}^d$, shape
parameter $\gamma \in R \setminus [0, 1]$, and positive definite scale parameter matrix  $\Sigma \in \mathbb{R}^{d\times d}$
when \pdf $p_{\vX}$ of $\vX$ is of the form 
\begin{equation}
    p_{\vX}(\vY)=p_{\vX}(\vY;\mu,\Sigma,\gamma,d):=C_{\vX}\exp\left \{-\frac{\gamma-1}{\gamma}Q_{\vX}(\vY)^{\frac{\gamma}{2(\gamma-1)}}\right\}, \quad \vY\in \mathbb{R}^d,
\end{equation}
where $Q_{\vX}$ is the $d$-quadratic form $Q_{\vX}(\vY):=(\vY-\mu)\cdot \Sigma^{-1}\cdot (\vY-\mu)^T$, 
\begin{equation}
\label{eq:cov-gamma-GND}
C_{\vX}:=C_{\vX}(\Sigma,\gamma,d):=\frac{\Gamma(d/2+1)}{\pi^{d/2}\Gamma\left( d\cdot{\frac{\gamma-1}{\gamma}}+1 \right)\sqrt{\vert \Sigma \vert}} \left (\frac{\gamma-1}{\gamma}\right )^{d\frac{\gamma-1}{\gamma}}.
\end{equation}
Note, that $\gamma=2$ is equivalent to the multivariate normal distribution. 

% The KLD formula is analytically known. Let $X\in \mathcal{N}_{\gamma}(\mu_1,\sigma_1^2I_p)$ and $Y\in \mathcal{N}_{\gamma}(\mu_2,\sigma_2^2I_p)$, with $\mu=\mu_1=\mu_2 \in \mathbb{R}^{d}$, the KLD from $Y$ to $X$ is 
% \begin{equation}
% \label{eq:KLDgamma}
%     D_{KL}(X\Vert Y)=d\log \frac{\sigma_2}{\sigma_1} - d\left (\frac{\gamma-1}{\gamma}\right)\left [ 
%     1-\left(\frac{\sigma_1}{\sigma_2}\right )^{\frac{\gamma}{\gamma-1}}
%     \right].
% \end{equation}

\end{example}
\AL{Further we compute distances $D_{KL}$ and $D_{H^2}$ between $\gamma=2$-GND and $\gamma=3$-GND. The mean values and matrices $\Sigma$ are assumed to be equal. All Tables as in previous example. TODO}
\begin{table}[h]
 \centering
 \begin{tabular}{|l|l|l|l|}
 \hline
Name of the divergence & Tensors & MC & Analytical \\ \hline \hline
Kullback–Leibler-(KL) --- $D_{\text{KL}}(\mathcal{N}_1\vert \mathcal{N}_2)$: && &$90.5559$\\ \hline
squared Hellinger distance --- $D_{H^2}(\mathcal{N}_1\vert \mathcal{N}_2)$: &&& \\ \hline
entropy $h(p)$ &&& \\ \hline
%Bregman divergence  --- $D_{\phi}$:	&&&\\ \hline
%Bhattacharyya distance --- $D_{\text{Bh}}$: &&& \\ \hline
\end{tabular}
 \caption{Comparison of KLD and entropy computed via low-rank tensors and MC methods, and by analytical formulas respectively. \ALc{TO BE DONE. COMPUTE TIME}}
 \label{table:divergences-comput_gamma}  
\end{table}%

%
%
%\subsection{Other tests}
\begin{example}
 \AL{Settings like in the previous example, but $d=100$ (and not 2).}
\end{example}
%

% \begin{example}
% \AL{Similar settings as in two previous examples, but to use formulas 2.12, 3.11, 3.10abc and 3.12 from \cite{Toulias2020}.}
% \end{example}
 
\AL{MARCO: A nice formula for the Kullback-Leibler divergence between univariate Cauchy densities is presented in the expression (11) of the arXiv preprint (\url{https://arxiv.org/abs/1905.10965}).}
 
\AL{MARCO: A closed-form expression of the Kullback-Leibler divergence between two univariate Weibull distributions is presented in p.4756 of the enclosed reference 2019Weibull statistical modeling for textured image retrieval.pdf}
 
\AL{MARCO: The closed-form expression of the Kullback-Leibler divergence between two zero-mean multivariate generalized Gaussian distributions (defined in (1), p.1021, please see the enclosed reference 2019KLD between MGGDs.pdf) is presented in (4), p.1022.}
 
\AL{MARCO: A closed-form of the Kullback-Leibler divergence between two multivariate generalized Gamma distributions (density defined in (8), p.224, see the enclosed reference 2015multivariate model for color texture classification.pdf) is presented in (15), p.226.
}


\begin{example}
????Take $d=100$. Generate a vector of size $2^d$ with entries $\{1,\ldots,2^d\}$ ????. Reshape this vector in a $d$-dimensional tensor $\tnb{w}$ of size $2^d$. We use the TT-cross algorithm (with accuracy $10^{-12}$) to compute a low-rank tensor approximation of $f(\tnb{w})=\sqrt{\tnb{w}}$. We observe that the TT ranks are equal 2. After 7 iterations the approximation error is $7.06e-13$. The computing time is $0.27$ seconds. For additional control we approximate numerically the integral $\int_0^1 \sqrt{x} dx$ on a grid with $2^d$ steps. The analytical solution is known and is $\frac{2}{3}$.\\
%
The same we did with $f(\tnb{w})=\log(1+\tnb{w})$. We approximated it with the TT-cross. After 7 iterations the approximation error is $8.46e-14$, the computing time is $0.22$ seconds.
The numerical integration of the integral $\int_0^1 \log(1+x) dx = 2\cdot \log(2)-1$ gives error $2.2e-15$.


In the next experiment we took again the same tensor $\tnb{w}$. The next function which we investigated is $f(\tnb{w})=\exp{(-\tnb{w}.*\tnb{w})}$. After 7 iterations the approximation error is $9.8e-14$. The computing time is $0.25$ seconds.
The analytical integral value is known $\int_0^1 e^{-x^2} dx \approx 0.74682413281$. The approximation on a grid with $2^d$ nodes gives the integration error $2.4e-12$. 
\end{example}
%
\begin{example}
%[Approximation of $d$-variate Gaussian \pdf]
Consider two Gaussian distributions  $\mathcal{N}_1:=\mathcal{N}(\mu_1,\bC^{(1)})$ and $\mathcal{N}_2:=\mathcal{N}(\mu_2,\bC^{(2)})$, where $\mu_1=(5.0\ldots,5.0)$ and $\mu_2=(6.1,\ldots, 6.1)$,
and non-singular covariance matrices $\bC^{(1)},\,\bC^{(2)}\in\mathbb{R}^{d\times d}$ such that:
both matrices are tridiagonal
with $\bC^{(1)}_{i,i}=4$, and $\bC_{i,j+1}=1$, $\bC_{i+1,j}=1$, and $\bC^{(2)}=2.1\cdot \bC^{(2)}$ for all $1\leq i,j\leq d$, $d=200$. The entropy and KLD computed via low-rank tensor and MC methods, and via the well-known analytical formulas are summarized in Table~\ref{table:divergences-comput0}.
The number of MC samples is $M=10^4$. 

Let 
$\vX=(\xi_1,\xi_2,...,\xi_d)$  be a $d$-dimensional Gaussian random vector with \pdf $p_{\vX}(\by)$. Then
$p_{\vX}(\by)$ is analytically separable and is expressed as a product of $d$ uni-dimensional densities:
\begin{equation}  \label{eq:motiv_inv2}
p_{\vX}(\by)=p _{\xi_1}(y_1) \cdot ... \cdot p_{\xi_d}(y_d),\quad \by:=(y_1,\ldots,y_d) \in \D{R}^d.
\end{equation}
\end{example}

The \emph{differential entropy} \refeq{eq:discr-diff-entrop}, requiring the 
point-wise logarithm of $p$, will be:
\begin{align*} 
   h(p) &:= \EXP{-\ln(p_{\vX}(\by))} = \EXP{-\ln(p_{\xi_1}(y_1) \cdot ... \cdot p_{\xi_d}(y_d))}=-\sum_{\nu=1}^d \EXP{\ln(p_{\xi_{\nu}}(y_{\nu}))}.
%   &=-\EXP{\log(p_{\xi_1}(y_1)) }- \ldots - \EXP{\log(p_{\xi_d}(y_d))}.
\end{align*}
i.e. for the $d$-dimensional Gaussian case, the differential entropy is a sum of one-dimensional entropies. The well-known formula for computing differential entropy of $d$-dimensional Gaussian random vector is:
\begin{equation*}
    \hat{h}(p)=\frac{d}{2}+\frac{d}{2}\ln(2\pi)+\frac{d}{2}\ln(|\bC|).
\end{equation*}
% This example with analytically known entropy is useful to demonstrate the whole approach. After estimating \pdfs from \pcfs, computing point-wise logarithms, we should obtain $h(p)\approx \hat{h}(p)$.\\

\begin{table}[h]
 \centering
 \begin{tabular}{|l|l|l|l|}
 \hline
Name of the divergence & Tensors & MC & Analytical \\ \hline \hline
Kullback–Leibler-(KL) --- $D_{\text{KL}}(\mathcal{N}_1\vert \mathcal{N}_2)$: &&$90.8098$ &$90.5559$\\ \hline
squared Hellinger distance --- $D_{H^2}(\mathcal{N}_1\vert \mathcal{N}_2)$: &&& \\ \hline
entropy $h(p)$ &&$415.58$&$415.52$ \\ \hline
%Bregman divergence  --- $D_{\phi}$:	&&&\\ \hline
%Bhattacharyya distance --- $D_{\text{Bh}}$: &&& \\ \hline
\end{tabular}
 \caption{Comparison of KLD and entropy computed via low-rank tensors and MC methods, and by analytical formulas respectively. \ALc{TO BE DONE. COMPUTE TIME}}
 \label{table:divergences-comput0}  
\end{table}
%
\subsection{New example, Sept 2021}
\textcolor{red}{New example, Sept 2021}
\begin{example}[Non-Gaussian \pdfs]
Let $\tnb{w}_1$ and $\tnb{w}_1$ be two random tensors, and $\tnb{v}$ a tensor obtained after discretisation of the multivariate Gaussian \pdf. To generate two tensors for non-Gaussian \pdfs, we compute the following steps:\\
1) the Hadamard product $\tnb{z}_i:=(\tnb{w}_i\odot \tnb{v})$ to get a tensor which contains small (decaying) elements in the ``far field'';\\
2) $\tnb{z}_i^{\odot 2}$ to make this tensor positive; and \\
3) scale them so that it behaves like a \pdf function, i.e., the integral of it should be one. Denote the scaled tensors by $\tnb{P}$ and $\tnb{Q}$.\\
\textcolor{red}{TODO We compute the differential entropy of each, the KLD divergence, and the Hellinger distance between them. Describe every steps, $\log$, Hadamard inverse, expected value... see Table 2? in Sect 4?.}
For all these steps, we demonstrate the tensor ranks and computing times.
\end{example}

% \begin{equation}  \label{eq:discr-int-qoi-g}
%  \EXP{\vek{g}_{\nu}}= \int_{\Rd} \vek{g}(\bx) p_{\vX}(\bx)\, \di \bx \; \approx \;
%   \D{E}_{\C{T}}(\tnb{G}) =  \frac{1}{N} \bkt{\tnb{G}}{\tnb{P}}_{\C{T}} .
% \end{equation}

% , assume that in the above example the data has
% been stored in the matrix $\vek{W}\in\D{R}^{M\times M}$, where $M=10^8=\sqrt{N}$,
% and consider its singular value decomposition (SVD)
% $\vek{W}=\vek{U}\vek{\Sigma}\vek{V}^\trpos = \sum_{m=1}^M \vsigma_m \vek{u}_m \vek{v}_m^\trpos$,
% where  $\vek{\Sigma}=\diag(\vsigma_1,\dots,\vsigma_M)$ is the diagonal matrix
% of singular values $\vsigma_m\ge 0$, assumed arranged by decreasing value,
% and $\vek{U}=[\vek{u}_1,\dots,\vek{u}_M]$,
% $\vek{V}=[\vek{v}_1,\dots,\vek{v}_M]$ collect the right and left singular vectors.
% Often there is a number $r\ll M$, such that for some small $\vepsilon>0$ one has
% $\vsigma_m \le \vepsilon$ for all $m>r$. Then one can formulate a compressed or
% truncated version 
% \[
% \vek{W}\approx\vek{W}_r =\vek{U}_r\vek{\Sigma}_r\vek{V}_r^\trpos
% =\sum_{m=1}^r \vsigma_m \vek{u}_m \vek{v}_m^\trpos
% =\sum_{m=1}^r  \vek{w}^{(1)}_m \otimes \vek{w}^{(2)}_m,
% \] 
% where $\vek{\Sigma}_r=\diag(\vsigma_1,\dots,\vsigma_r)$,
% $\vek{U}_r=[\vek{u}_1,\dots,\vek{u}_r]$, $\vek{V}_r=[\vek{v}_1,\dots,\vek{v}_r]$,
% and $\vek{w}^{(1)}_m = \sqrt{\vsigma_m} \vek{u}_m$, $\vek{w}^{(2)}_m = \sqrt{\vsigma_m} \vek{v}_m$.

%Another difference between tensors and matrices is that a
%matrix has only one rank, whereas a tensor may have many ranks. (obtained, for instance, 
%after the discretization 
%of a function $f(\bx,\by)=f(\vert \bx-\by\vert)$) separates a point $\bx=(x_1,...,x_d)\in \mathbb{R}^{d}$ from 
%a point $\by=(y_1,...,y_d)\in \mathbb{R}^{d}$, whereas the corresponding tensor (depending on tensor format) 
%separates $x_1-y_1$ from $x_2-y_2$... and $x_d-y_d$. This implies that tensors may have $d$ ranks $\br=(r_1,\ldots,r_d)$. In such case we speak about \textit{tensor rank}. 

%  $Log: appendix.tex,v $
%  Revision 1.10  2021/08/03 08:24:00  hgm
%  small changes
%
%  Revision 1.8  2021/04/17 09:50:41  hgm
%  include -> input
%
%  Revision 1.7  2021/04/16 21:41:34  hgm
%  changes acc. to protocol of Apr 2021
%
%  Revision 1.1  2019/06/10 22:08:54  hgm
%  further down the road
%
%  $Log: appendix.tex,v $
%  Revision 1.10  2021/08/03 08:24:00  hgm
%  small changes
%
%  Revision 1.8  2021/04/17 09:50:41  hgm
%  include -> input
%
%  Revision 1.7  2021/04/16 21:41:34  hgm
%  changes acc. to protocol of Apr 2021
%
%  Revision 1.6  2019/06/10 01:22:05  hgm
%  runs
%
%  Revision 1.5  2019/06/09 10:28:17  hgm
%  for new article
%
%  Revision 1.4  2019/05/27 23:28:20  hgm
%  tiny correction
%
%  Revision 1.3  2019/04/13 18:43:03  hgm
%  describes notation
%
%  Revision 1.2  2019/04/13 10:30:57  hgm
%  little changes, shifted fonts
%
%  Revision 1.1  2019/03/08 23:24:43  hgm
%  initial check-in
%
%
%
%
%



%%% Local Variables: 
%%% mode: latex
%%% TeX-master: "../19_low-rank_tensor_prob_den_char"
%%% End: 
